# Supplementary material for: IBIA: Bayesian Inference via Incremental Build-Infer-Approximate operations on Clique Trees
Source: arXiv:2202.12003 source file (2022-08-10)
Supplement: Supplementary file 1 [file appendix2.tex]

%\section{Detailed results}\label{app:bnuai}
%In this section, we show detailed results obtained with FBP, WMB, IJGP and IBIA for a subset of the BN\_UAI benchmarks. 
%
%Table~\ref{tab:pr.bnuai.ace} tabulates error in $\log(PR)$. 
%Benchmarks for which all methods give accurate results are not included here.
%It is seen from the table that IBIA has a mean error of the order of $10^{-6}$ and maximum of $10^{-5}$, both of which are several orders of magnitude lower than the other methods. Further, although the mean errors obtained with FBP is of the order of $10^{-1}$, the errors for some testcases like BN\_24, BN\_25 are as large as $4$. Although the bound obtained with WMB is good in many cases, it is worse than the LBP variants for BN\_30-40. There are also many cases for which the estimates obtained by WMB are greater than one, which are marked with a dash in the table. 
%
%Table~\ref{tab:postmar.bnuai.ace.abs} compares the maximum error and RMSE in $MAR_e$ obtained with different inference algorithms. We present results obtained with two sets of clique size constraints: $mcs_p = 20, ~mcs_{im} = 15$ and $mcs_p = 15, mcs_{im} = 10$. 
%It is seen from the table that IBIA results in the least average max-error and RMSE compared to other methods for both sets of clique size constraints. 
%As discussed, an error of zero, means that the error is less than $0.001$. 
% When $mcs_p$ is reduced to 15, both max-error and RMSE increase, but continue to be lower than other methods for most cases. The maximum error is around 0.1 or lower in all cases except BN\_59, BN\_60, where it increases to 0.45 and 0.62 which is comparable to the error obtained using the other methods. Testcases BN\_90 and BN\_91 could not be inferred with $mcs_p=15$, since the maximum CPD size  is 17 (which is greater than $mcs_p$).
%
%Table~\ref{tab:runtimePosteriorBN} compares the runtime required for inference of $MAR_e$ using different methods. 
%Though runtimes for different methods are not directly comparable since they are implemented in different programming languages, it gives a decent overall idea. We note that even though IBIA is implemented in Python, the runtimes are quite competitive when compared to other tools. It is better than WMB and IJGP for all benchmarks.
%It is  faster than FBP for benchmarks with maximum in-degree between 5-19 (e.g., BN\_105, BN\_107, BN\_86, BN\_87, BN\_90, BN\_91). Our runtimes are also an order of magnitude lower than ACE for some benchmarks like BN\_14, BN\_2, BN\_8, BN\_86, etc.
%
%Table~\ref{tab:priormar.bnuai.ace.abs} has the maximum error, the RMSE, and the runtime required for inference of $MAR_p$. 
%Benchmarks for which all methods give accurate results are not included here. 
%Once again, both the average max-error and RMSE obtained with IBIA are an order of magnitude lower than with other methods. Even though the number of CTFs in the sequence increases when compared to posteriors due to reduced simplifications, the max-error is larger than 0.05 only in six cases, and even here it is about 0.1. 
%In many cases, the runtime required for IBIA is orders of magnitude smaller than ACE, WMB, and IJGP. This is also partially due to the setting of the $ibound$ parameter in WMB and IJGP.  It is also lower than FBP for cases with large factor sizes. 
%
%\input{tables/pr.bnuai.ace.tex}
%\input{tables/postmar.bnuai.ace.abs.tex}
%\input{tables/postmar.bnuai.runtime.tex}
%\input{tables/priormar.bnuai.ace.abs.tex}
%
%%%\textcolor{red}{\bf Move main points to Appendix}
%%
%%%It is seen from the table that IBIA has a mean error of the order of $10^{-6}$ and maximum of $10^{-5}$, both of which are several orders of magnitude lower than the other methods. Further, although the mean errors obtained with FBP are of the order of $10^{-1}$, the errors for some testcases like BN\_24, BN\_25 are as large as $4$. IJGP does not give PR, while WMB gives upper bounds for PR. Therefore, the errors obtained with WMB are always positive. Although the bound is good in many cases, it is worse than the LBP variants for BN\_30-40. There are also many cases  for which the estimates obtained by WMB are greater than one, which are marked with a dash in the table. 
%%\input{tables/pr.bnuai.ace.tex}
%%%%%% BN_UAI - PostMAR  - Errors & Runtime
%%%Table~\ref{tab:postmar.bnuai.ace.abs} compares the maximum error and RMSE obtained with different inference algorithms for a subset of BN\_UAI testcases for which exact solutions are available. Small networks where all methods give accurate results are not tabulated here. In order to see the effect of clique sizes used in IBIA, we present results obtained with two sets of clique size constraints: $mcs_p = 20, ~mcs_{im} = 15$ and $mcs_p = 15, mcs_{im} = 10$.
%% %\input{tables/postmar.bnuai.ace.abs.tex}
%%%An advantage of IBIA, which it shares with IJGP and WMB, is that we will automatically get exact inference when the maximum clique size is less than than $mcs_p$ parameter. This is seen in many cases, where a single partition in obtained. With $mcs_p=15$, we get a lower number of such cases, as expected. With $ibound=20$, WMB and IJGP also perform exact inference for many of the networks (e.g., BN\_105, BN\_109, BN\_111). This is not possible in FBP and TRWBP, where the maximum errors are quite large in some cases. 
%%
%%%We note that both the maximum and RMS errors are significantly lower than other methods.  Even for testcases where there are 7-8 partitions (e.g., BN\_63-BN\_68), both maximum and RMS error obtained with IBIA are less than 0.05 when $mcs_p=20$. Even with $mcs_p = 15$, there are only two benchmarks,  BN\_59, BN\_60, where the maximum error is 0.45 and 0.62, which is comparable to the error obtained using the other methods.
%%%Also notable is the low errors in BN\_22 and 23, where the maximum error is 0.03, inspite of the very number of partitions obtained with $mcs_{p}=15$. This is possible with IBIA, if the structure allows for a large fraction of exact marginalizations during the approximation.
%%
%%%Although many of the benchmarks have a large treewidth \cite{citefix}, the presence of evidence variables results in a significant degree of simplification. The effect of the large treewidth will be more apparent in the results of $MAR_p$, presented in the next subsection.
%%%It is seen from the table that IBIA results in the least average max-error and RMSE compared to other methods for both sets of clique size constraints. With $mcs_p=20$, the average max-error over all benchmarks is 0.008 and the average RMSE is 0.001, an order of magnitude lower than that achieved with other methods. The maximum error obtained with IBIA is 0.06, with zero error in a large number of cases.
%%%As discussed, an error of zero, means that the marginals are accurate to 3 decimal places.
%%
%%%When $mcs_p$ is reduced to 15, both max-error and RMSE increase, but continue to be lower than other methods for most cases. The maximum error is around 0.1 or lower in all cases except BN\_59, BN\_60, where it increases to 0.45 and 0.62 which is comparable to the error obtained using the other methods. Testcases BN\_90 and BN\_91 could not be inferred with $mcs_p=15$, since the maximum CPD size  is 17 ($> ~mcs_p$).
%%
%%%IBIA is expected to give lower errors than FBP, due to larger cluster sizes. However, it also gives significantly lower errors than WMB and IJGP which are run with comparable or larger cluster sizes. We also note that although max-errors are greater than 0.5 for quite a few cases with FBP, WMB and IJGP, the mean RMSE is less than 0.15. This indicates that a large percentage of nodes have small errors with all approximate techniques.
%%
%%%An advantage that IBIA shares with WMB and IJGP is that we will get exact inference when the cluster size is less than than $mcs_p/ibound$ parameter. This is seen in many cases for IBIA, where a single partition in obtained, and for some cases of WMB/IJGP. This is not possible in FBP, where the maximum errors are quite large in some cases. With $mcs_p=15$, we get a lower number of such cases as expected.
%%
%%%	\item In many cases, we have a single partition after simplification. This means that our method performs exact junction tree based inference. With $ibound=20$, we believe WMB and IJGP also perform exact inference for many of the networks (e.g., BN\_105, BN\_109, BN\_111). 
%%	%Testcases were all methods give errors $<0.001$ are not tabulated here.
%%	%\item The proposed method has more testcases that reduce to standard BP (e.g., BN\_30-BN\_41) than other methods. This indicates that for these testcases, our evidence-based simplification outperforms those used in other methods. 
%%	%The error increases because some of the evidence variables are added to later partitions when the clique size constraint is reduced, leading to approximations during backpropagation.	
%%%	\item Although max-errors are greater than 0.5 for quite a few cases with FBP, TRWBP, WMB and IJGP, the mean RMSE is less than 0.15. This indicates that a large percentage of nodes have small errors with all approximate techniques.
%%%\end{itemize}
%%%\input{tables/postmar.bnuai.runtime.tex}
%%%Table~\ref{tab:runtimePosteriorBN} compares the runtime required for inference of posteriors using different methods. Though runtimes for different methods are not directly comparable since they are implemented in different programming languages, it gives a decent overall idea. We note that even though IBIA is implemented in Python, the runtimes are quite competitive when compared to other tools. It is better than WMB and IJGP for all benchmarks. This is probably due to the setting of the $ibound$ parameter, which was set to get a fair comparison of the error. It is  faster than FBP for benchmarks with maximum in-degree between 5-19 (e.g., BN\_105, BN\_107, BN\_86, BN\_87, BN\_90, BN\_91). Our runtimes are also an order of magnitude lower than ACE for some benchmarks like BN\_14, BN\_2, BN\_8, BN\_86, etc.
%%
%% \input{tables/postmar.bnuai.ace.abs.tex}
%%\input{tables/postmar.bnuai.runtime.tex}
%%%%%% Prior MAR - BN\_UAI - error table
%%
%%
%%%Once again, both the average max-error and RMSE obtained with IBIA are an order of magnitude lower than with other methods. Even though the number of partitions is increased when compared to posteriors due to reduced simplifications, the max-error is larger than 0.05 only in six cases, and even here it is about 0.1. 
%%
%%%In many cases, the runtime required for IBIA is orders of magnitude smaller than ACE, WMB, and IJGP. Once again, this is also partially due to the setting of the $ibound$ parameter in WMB and IJGP.  It is also lower than FBP for cases with large factor sizes. 
%%
%%\input{tables/priormar.bnuai.ace.abs.tex}
